# Supplementary material for: Phase discovery with active learning: Application to structural phase transitions in equiatomic NiTi
Source: arXiv:2401.05568 source file (2024-01-10)
Supplement: Supplementary file 1 [file si.pdf]

# Supplementary Information for:
# Phase discovery with on-the-fly machine learning: Application to phase transitions in equiatomic NiTi

Jonathan Vandermause,[1,2,*] Yucong Miao,[2] Anders Johansson,[2] Joost J. Vlassak,[2] and Boris Kozinsky[2,3,†]

[1]*Department of Physics, Harvard University, Cambridge, Massachusetts 02138, USA*

[2]*John A. Paulson School of Engineering and Applied Sciences, Harvard University, Cambridge, MA 02138, USA*

[3]*Robert Bosch LLC, Research and Technology Center, Cambridge, MA 02139, USA*

[*] jonathan_vandermause@g.harvard.edu

[†] bkoz@seas.harvard.edu

## I. ADDITIONAL DATA ON TRAINING SIMULATIONS

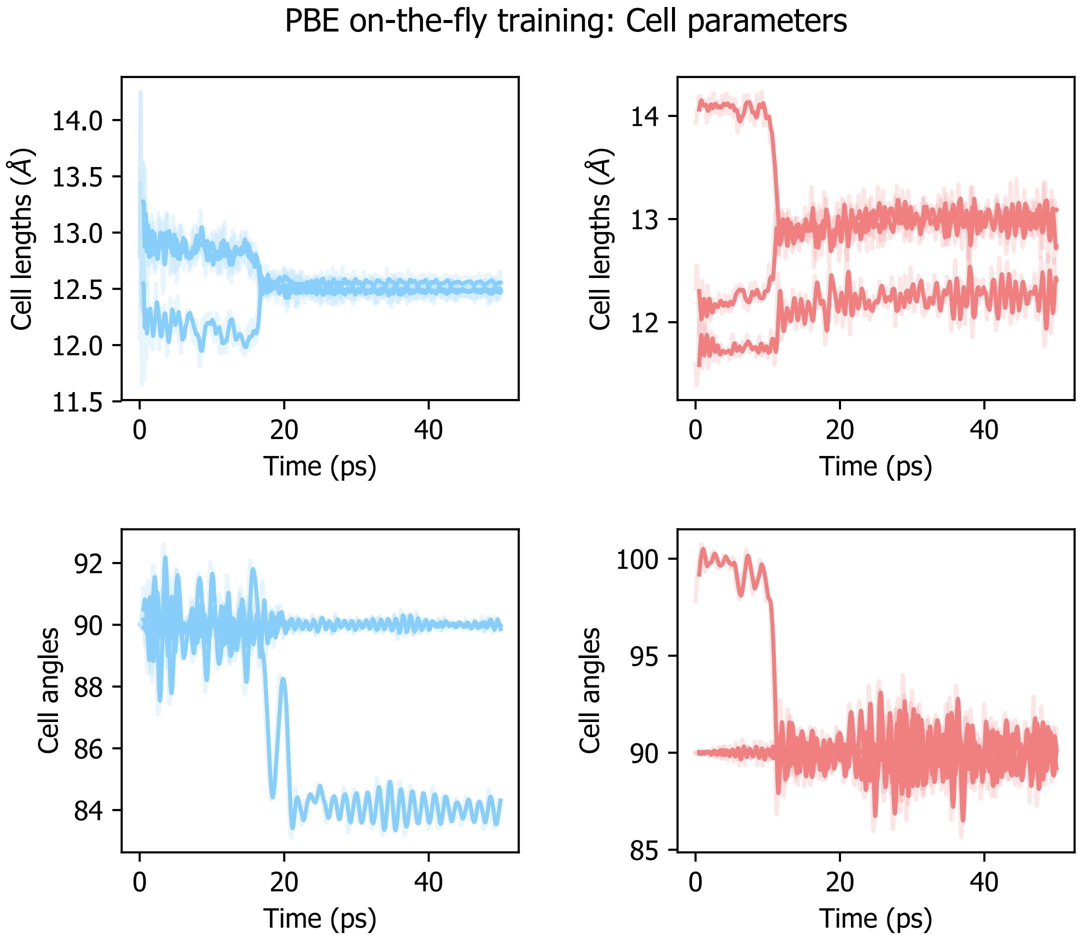


FIG. 1. Cell lengths and angles during PBE on-the-fly cooling and heating simulations.

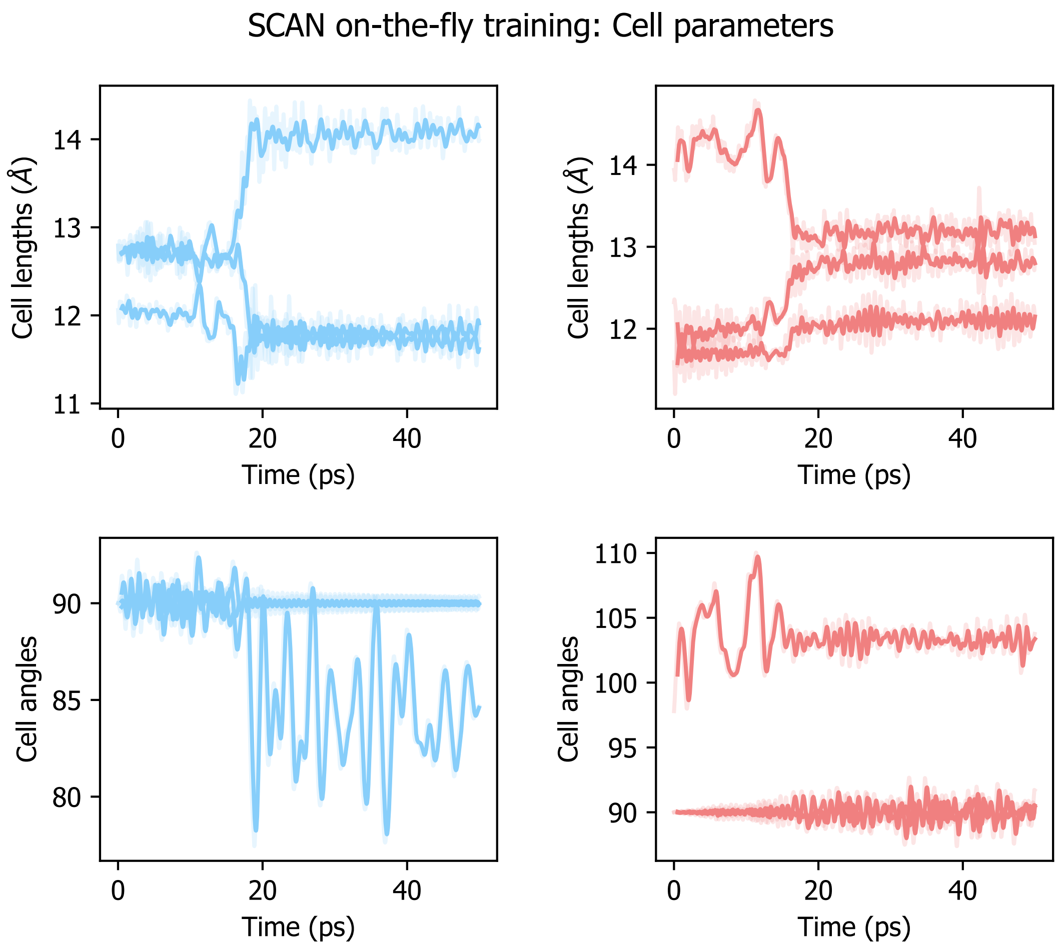


FIG. 2. Cell lengths and angles during SCAN on-the-fly cooling and heating simulations.

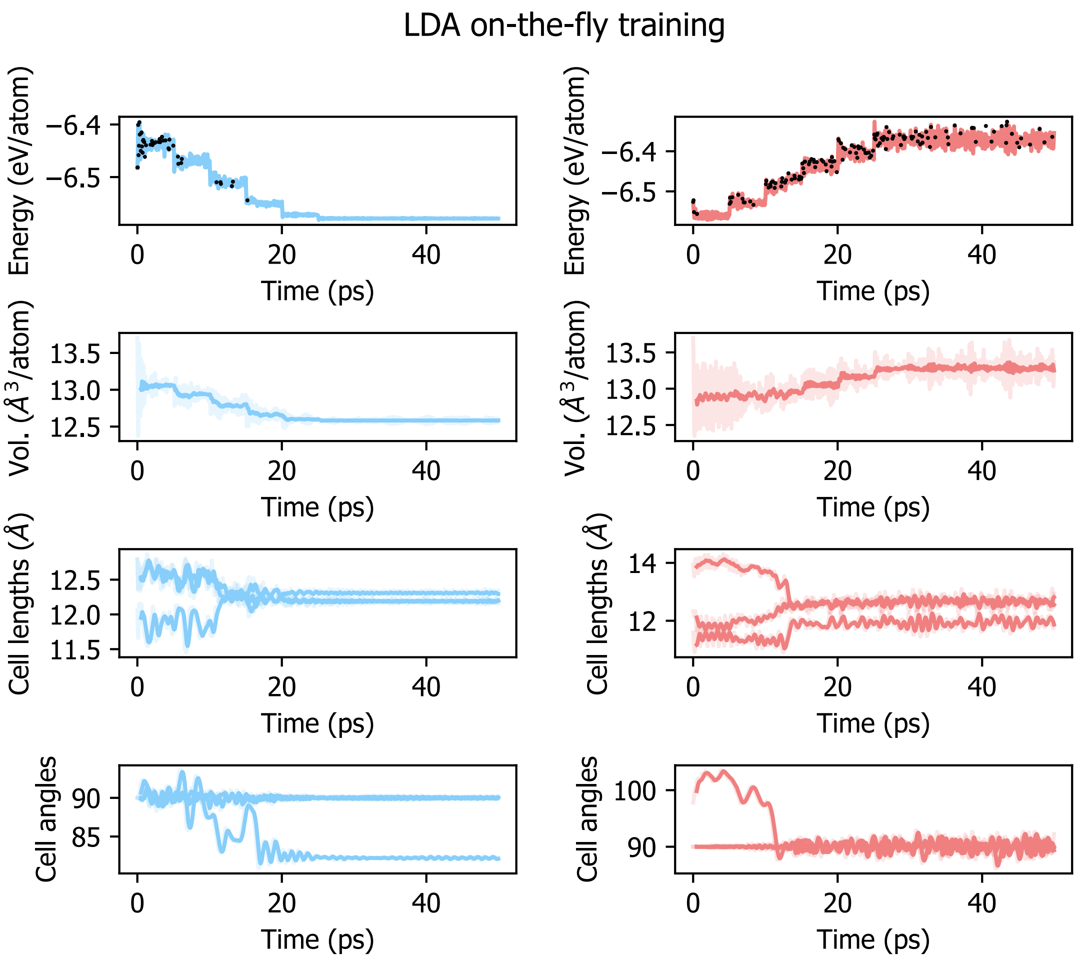


FIG. 3. Potential energies, atomic volumes, cell lengths and cell angles during LDA on-the-fly cooling and heating simulations.

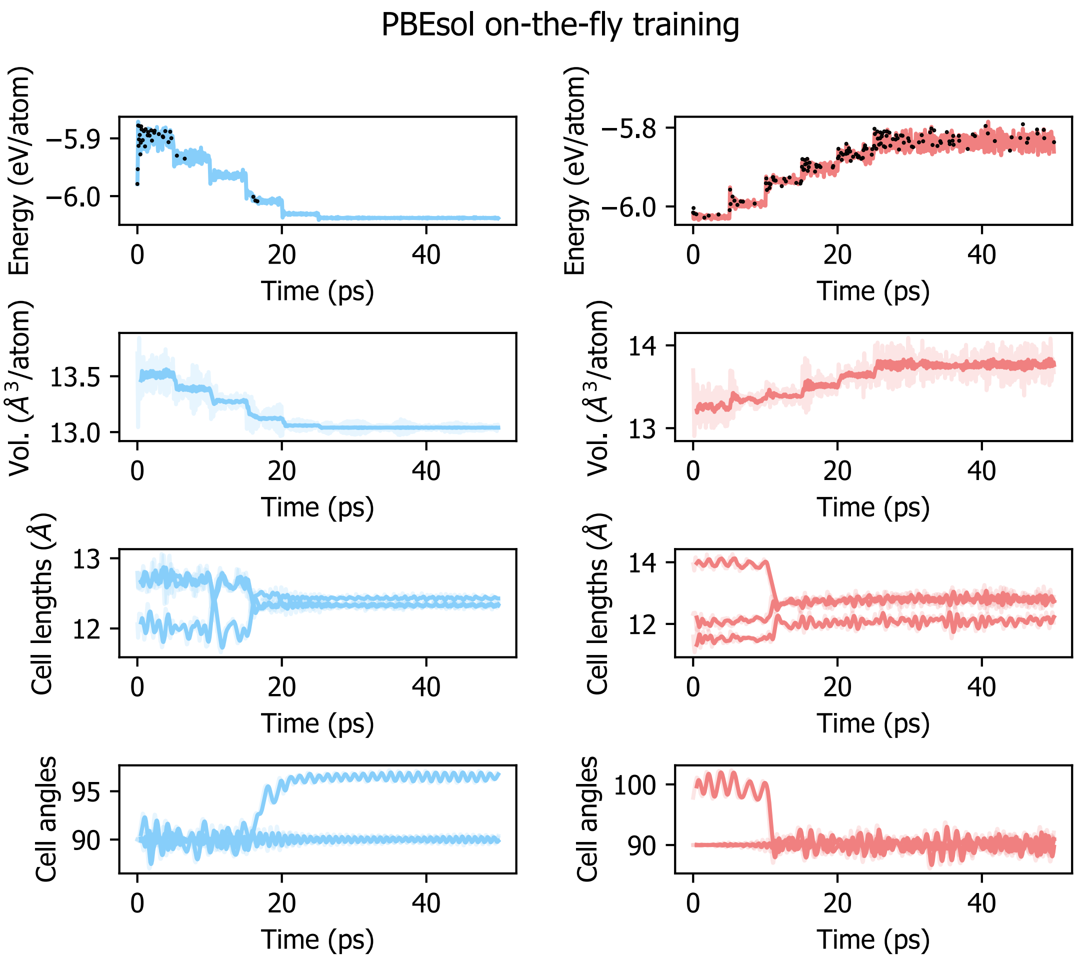


FIG. 4. Potential energies, atomic volumes, cell lengths and cell angles during PBEsol on-the-fly cooling and heating simulations.

## II. TRAINING ERRORS

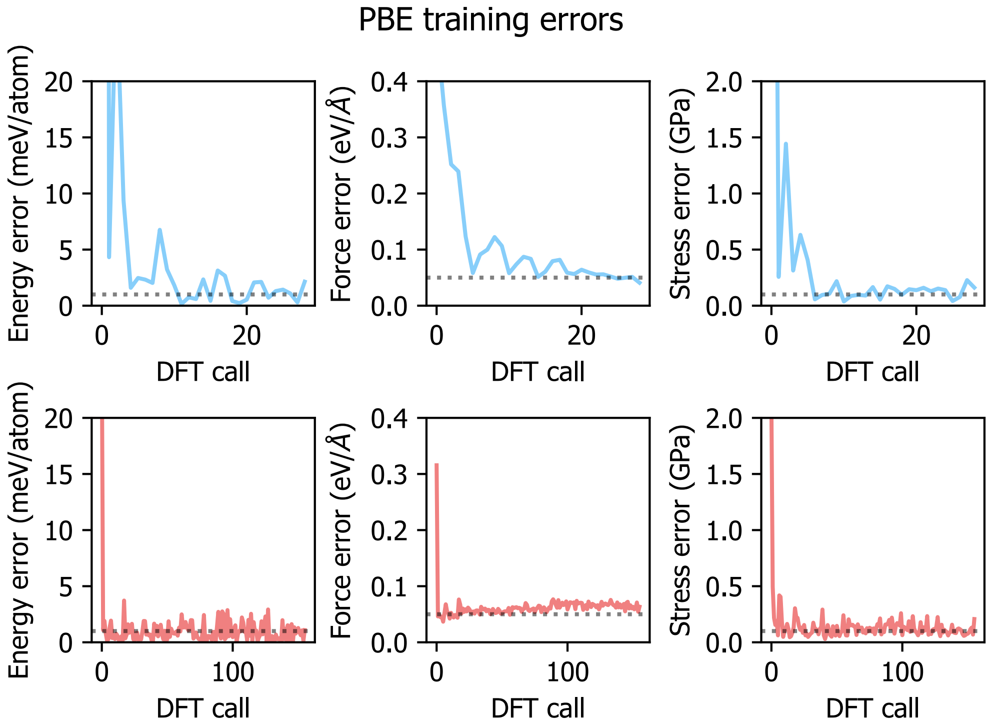


FIG. 5. Errors on energies, forces, and stresses during PBE training.

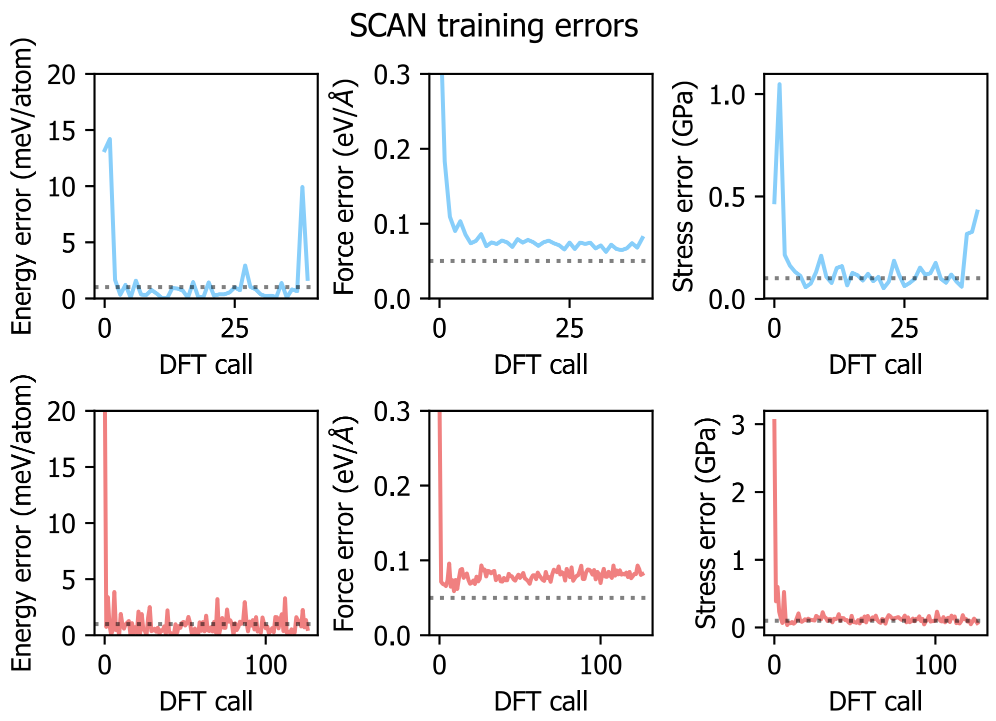


FIG. 6. Errors on energies, forces, and stresses during SCAN training.

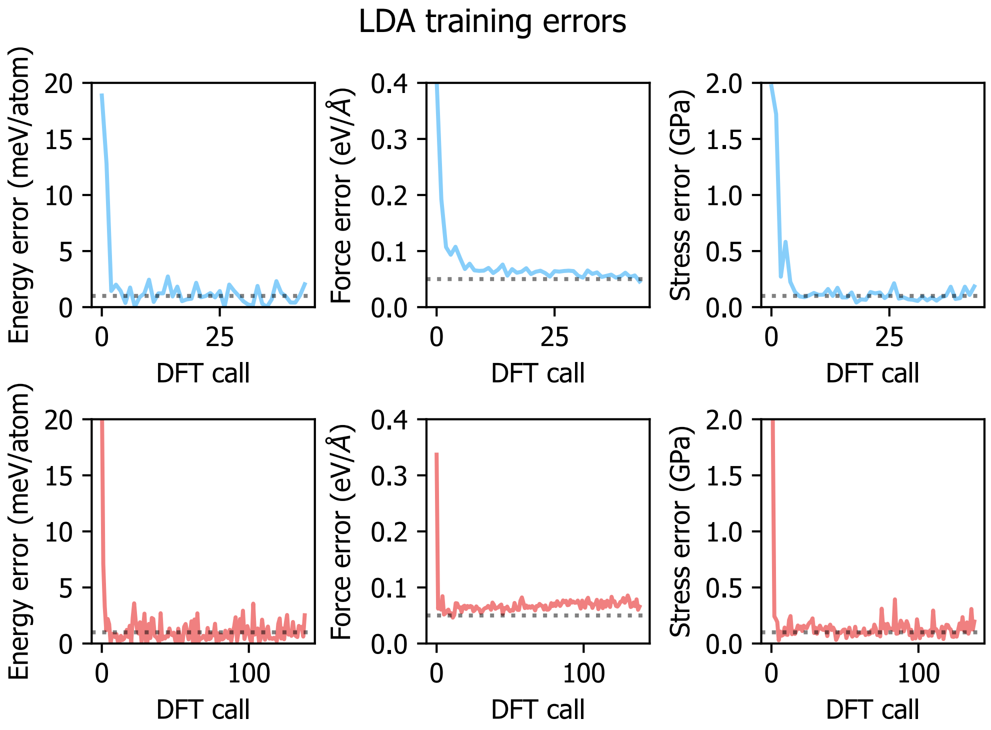


FIG. 7. Errors on energies, forces, and stresses during LDA training.

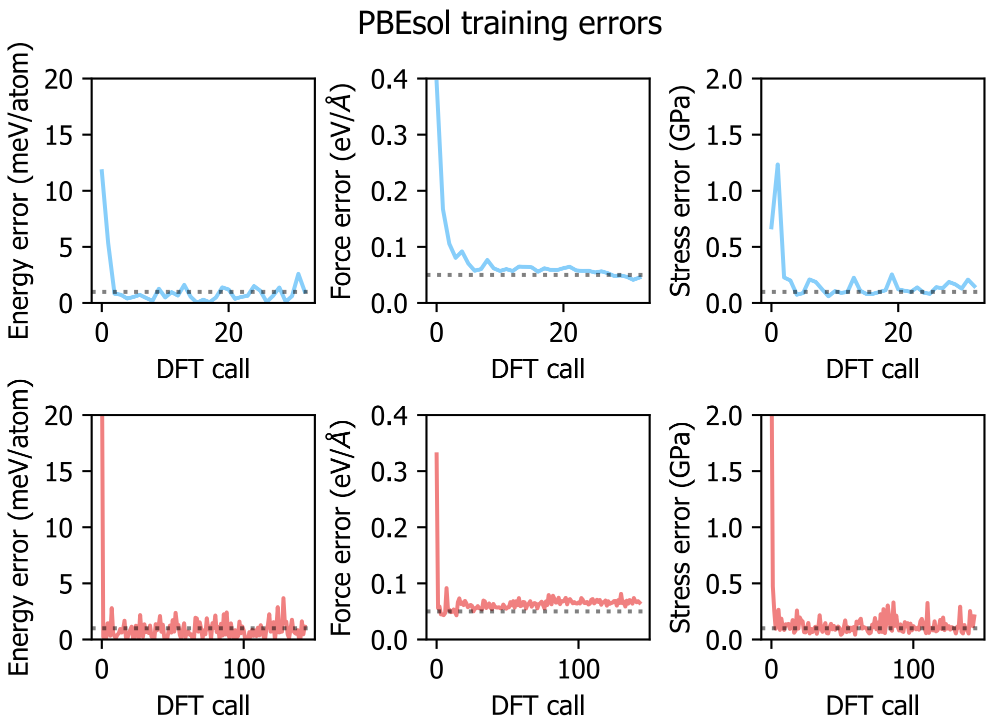


FIG. 8. Errors on energies, forces, and stresses during PBEsol training.

## III. VISUALIZATIONS OF COOLED NI-TI STRUCTURES

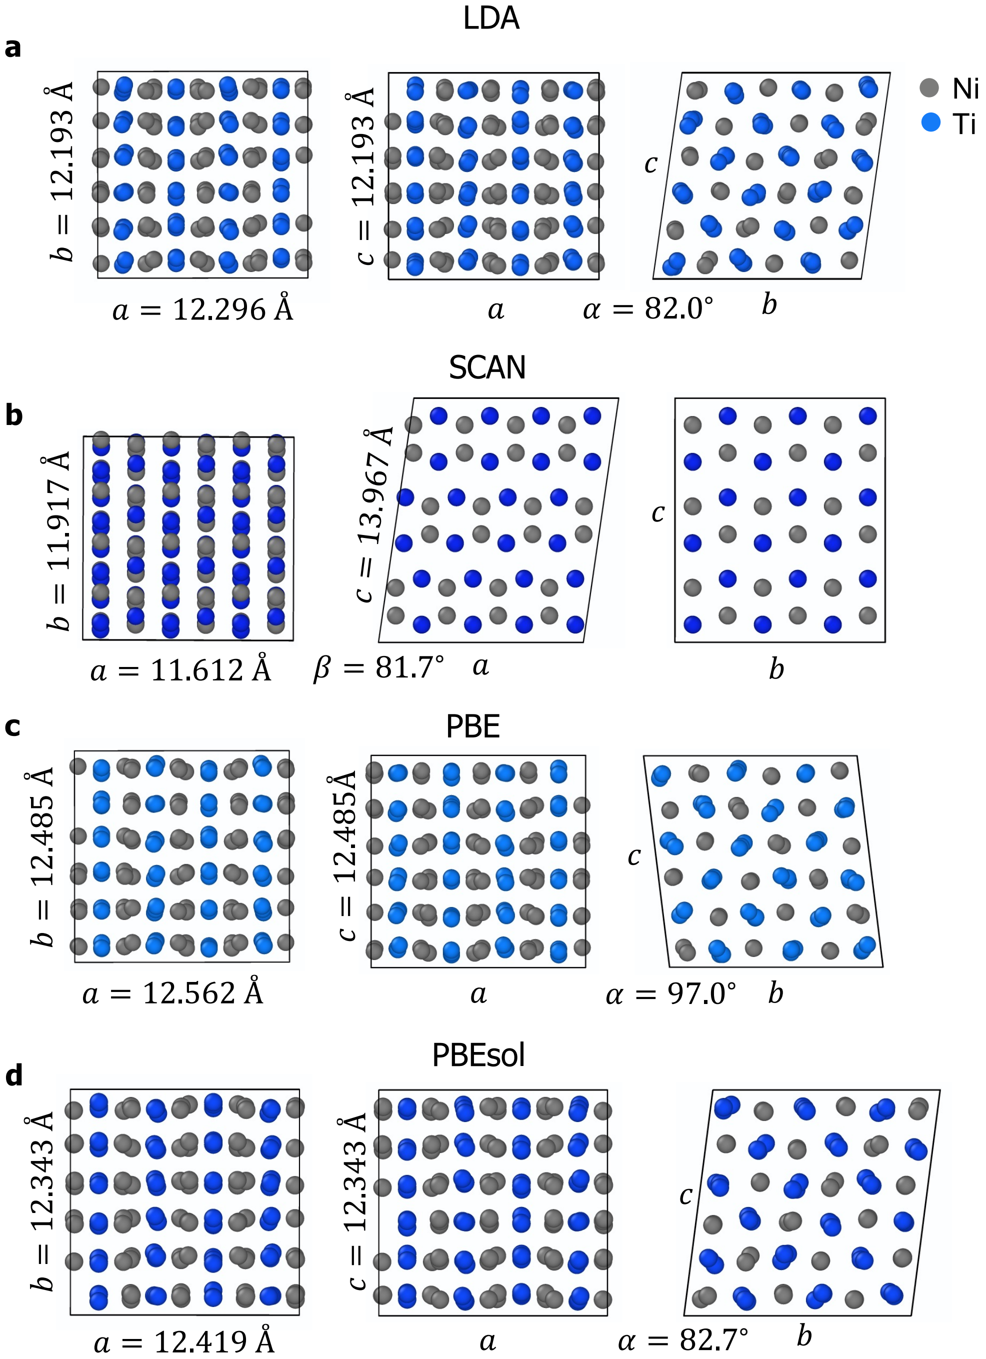


FIG. 9. Structures obtained from on-the-fly cooling simulations after relaxation of the atomic positions and unit cell.

## IV. ELASTIC CONSTANTS & PHONON FREQUENCIES

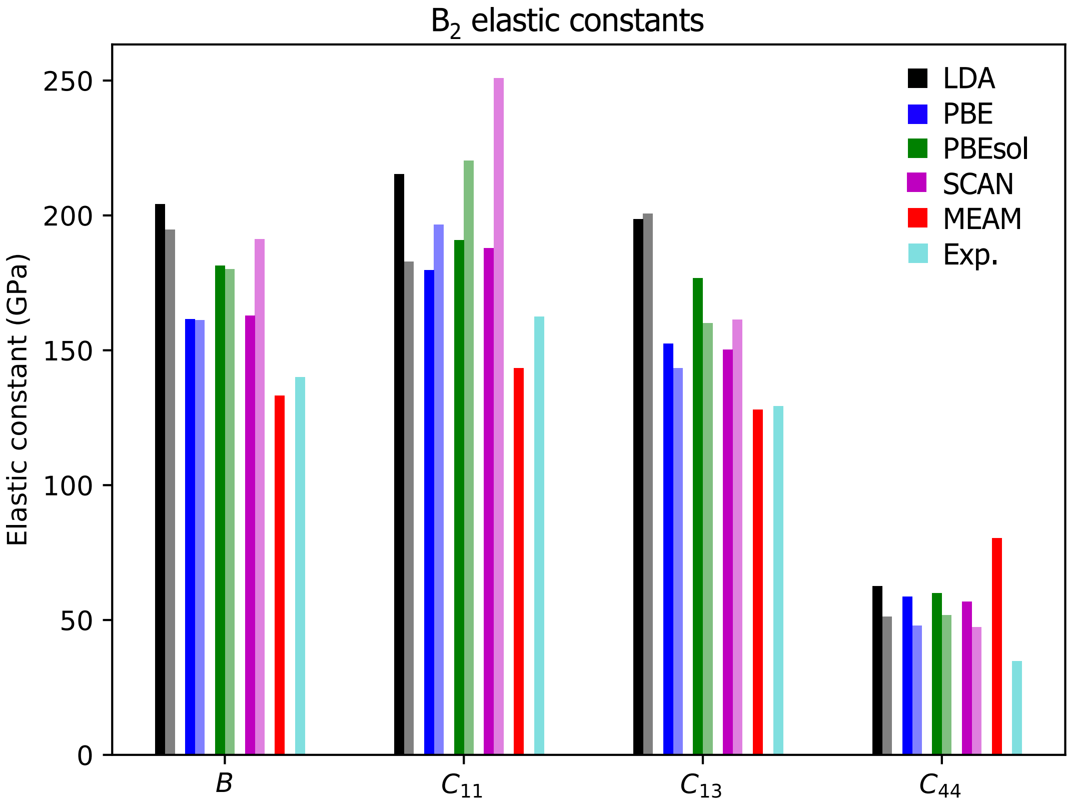


FIG. 10. $B2$ bulk modulus and elastic constants predicted by the four models trained in this work and the MEAM force field from [1]. Experimental measurements from [2] are shown in light blue.

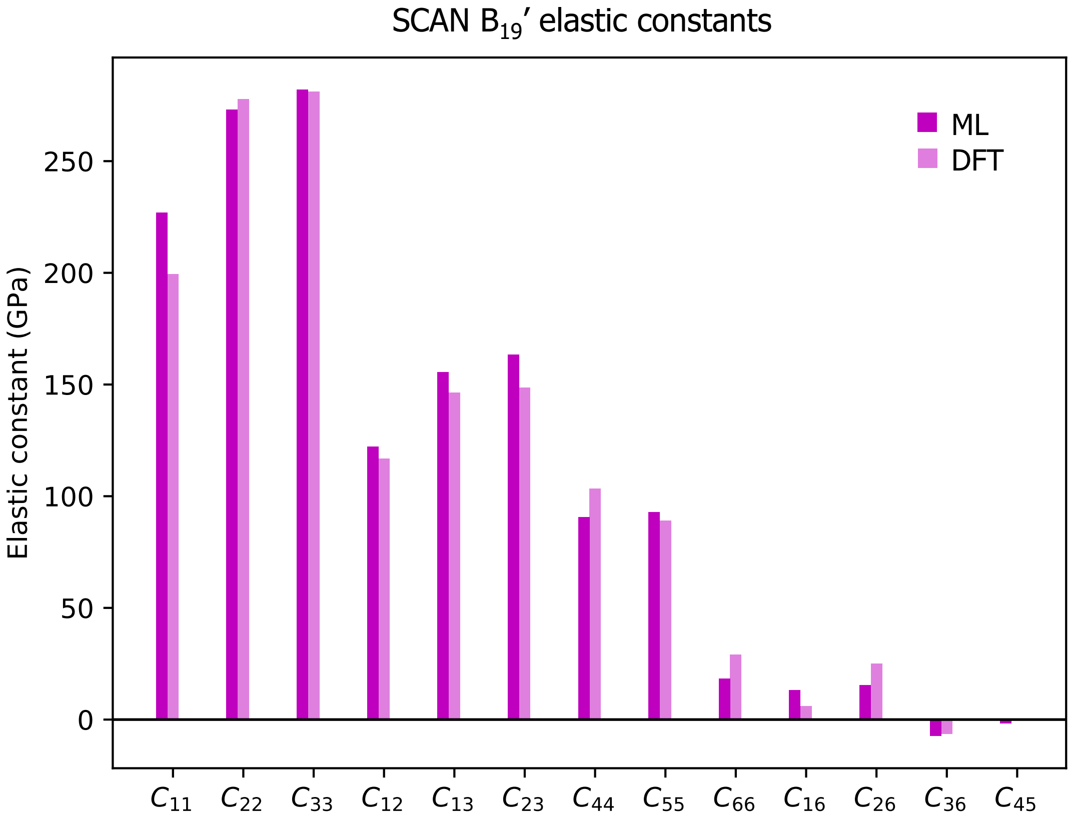
SCAN B19′ elastic constants
ML
DFT
Elastic constant (GPa)
250
200
150
100
50
0
C11
C22
C33
C12
C13
C23
C44
C55
C66
C16
C26
C36
C45

FIG. 11.

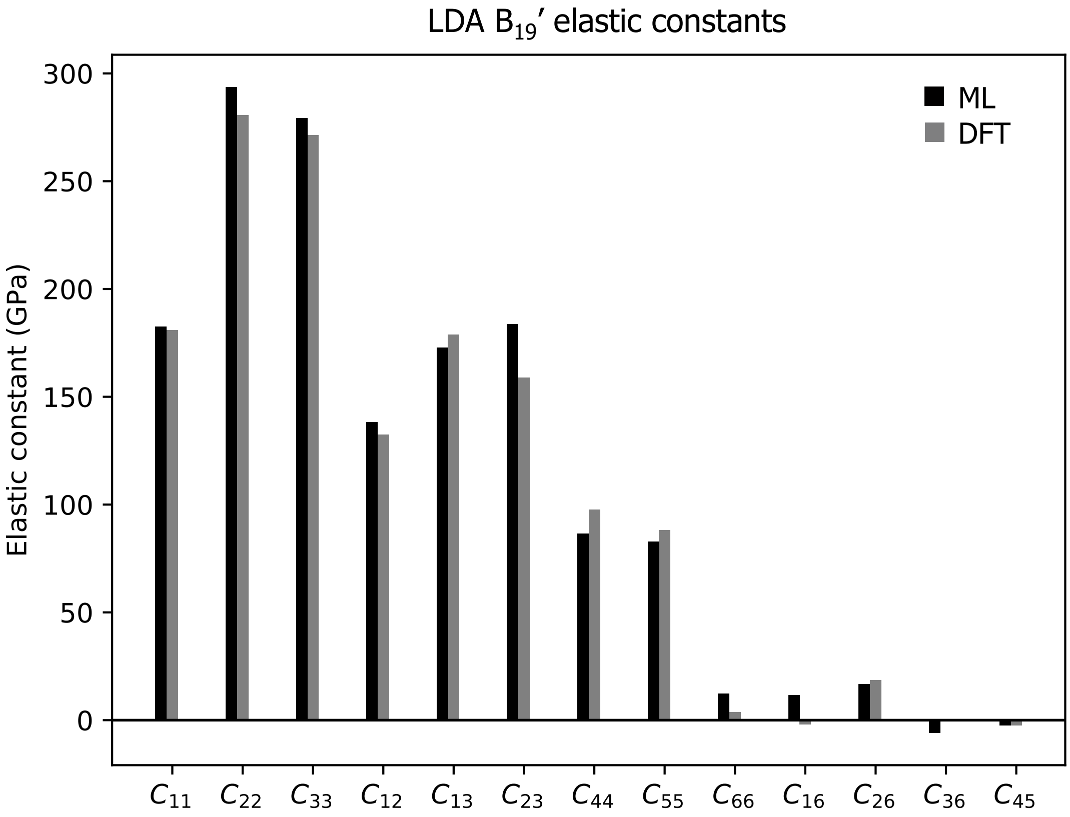
LDA B19′ elastic constants
ML
DFT
Elastic constant (GPa)
300
250
200
150
100
50
0
C11
C22
C33
C12
C13
C23
C44
C55
C66
C16
C26
C36
C45

FIG. 12.

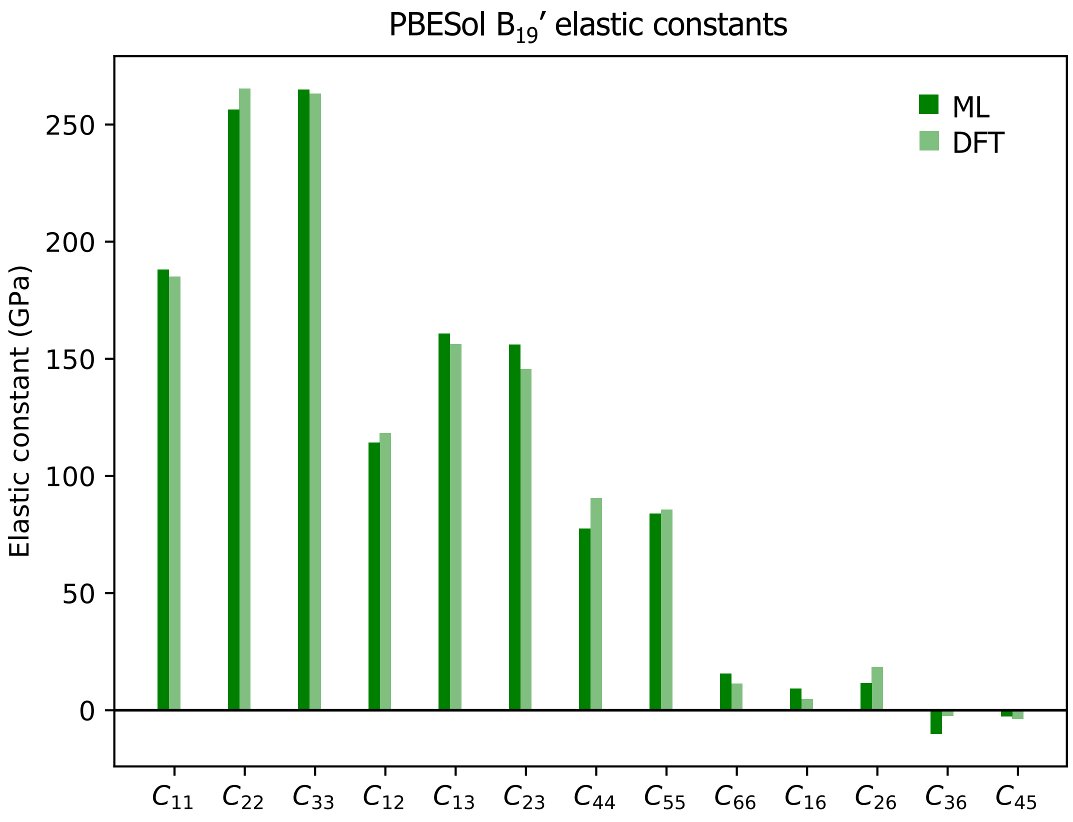


FIG. 13.

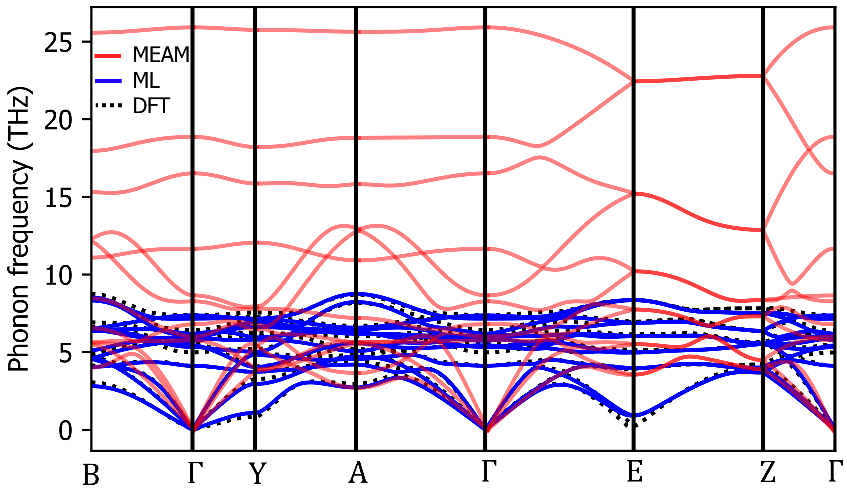


FIG. 14. $B19'$ phonons predicted by the PBE-trained model presented in this work (blue), PBE DFT (dotted), and the MEAM force field from [1].

## V. ADDITIONAL LARGE-SCALE MD DATA

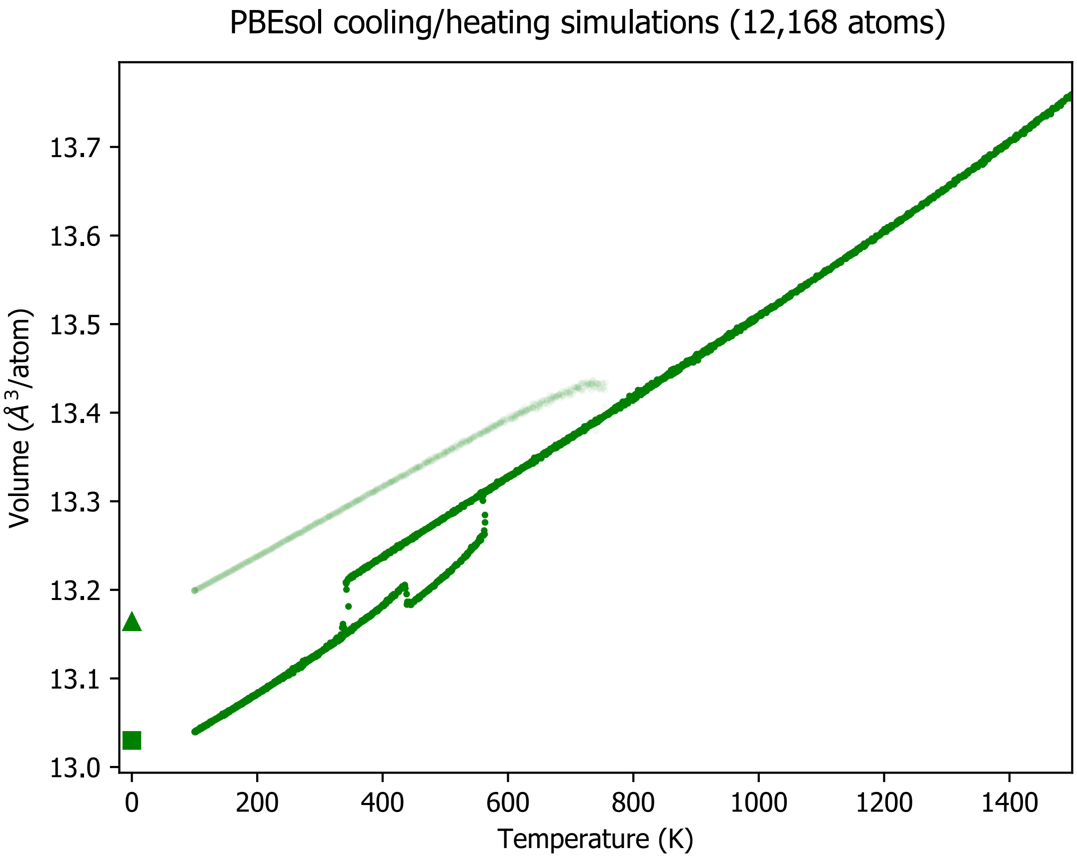


FIG. 15. Large-scale cooling/heating simulation of $B2$ (dark green) and heating simulation of $B19'$ (light green). Zero-Kelvin volumes of $B19'$ (triangle) and $M2$ (square) are shown for reference.

## VI. TEMPERATURE AND PRESSURE SWEEPS

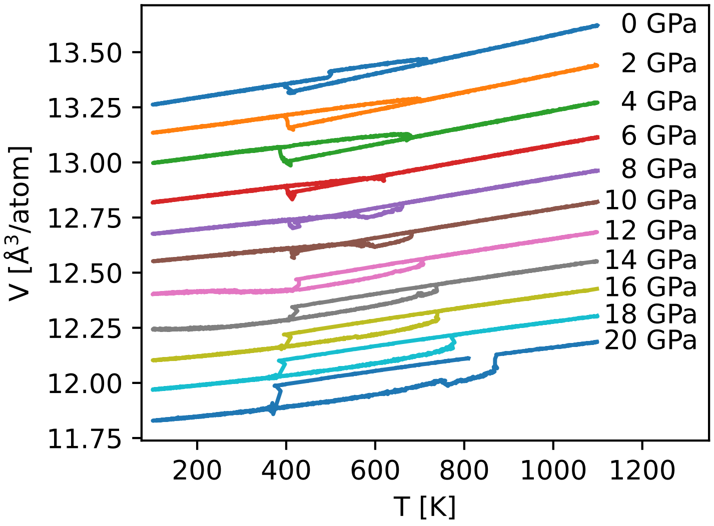


FIG. 16. Cooling/heating simulations with the SCAN force field at pressures ranging between 0 and 20 GPa, with a transition to a low-volume phase observed around 12 GPa.

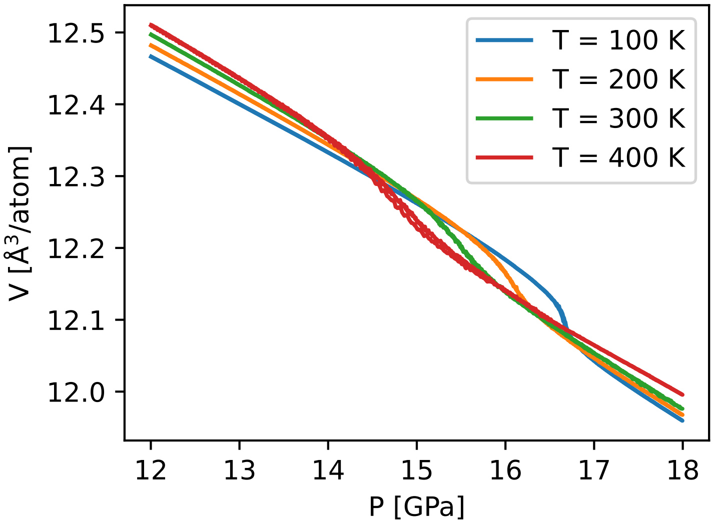


FIG. 17. Compression/decompression sweeps performed with the SCAN force field at temperatures ranging from 100 to 400 K. Simulations were initialized in a relaxed 9x9x9 $B19'$ supercell containing 105,000 atoms. Each system was equilibrated for 100 ps, compressed from 0 to 20 GPa for 2 ns, and finally decompressed from 20 to 0 GPa for 2 ns.

## VII. XRD SPECTRA

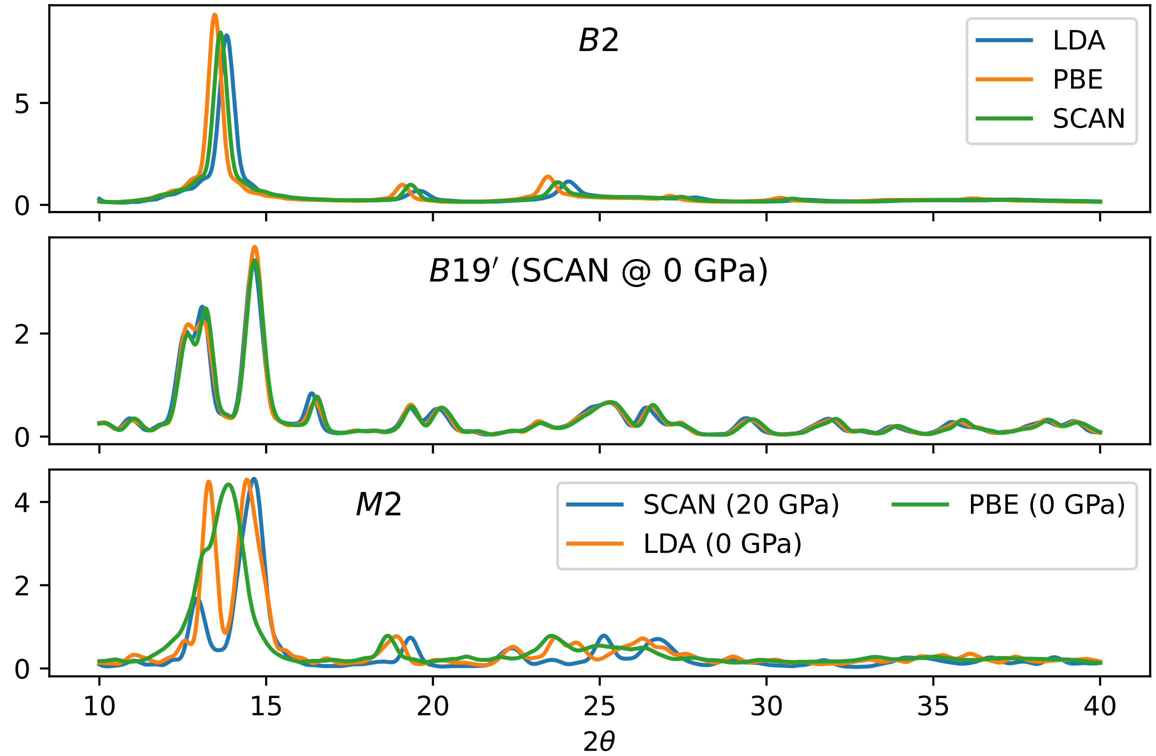


FIG. 18. Calculated XRD spectra with the LDA, PBE, and SCAN force fields in the $B2$ (top), $B19'$ (middle) and $M2$ phases (bottom). The different $B19'$ curves are different cycles from repeated compression/decompression. The spectra were computed using ASE [3] with Ni numbers added from [4] and simple GPU acceleration to allow large systems.

[1] Won-Seok Ko, Blazej Grabowski, and Jörg Neugebauer, "Development and application of a Ni-Ti interatomic potential with high predictive accuracy of the martensitic phase transition," Physical Review B **92**, 134107 (2015).

[2] O Mercier, KN Melton, G Gremaud, and J Hägi, "Single-crystal elastic constants of the equiatomic NiTi alloy near the martensitic transformation," Journal of Applied Physics **51**, 1833–1834 (1980).

[3] Ask Hjorth Larsen, Jens Jørgen Mortensen, Jakob Blomqvist, Ivano E Castelli, Rune Christensen, Marcin Dułak, Jesper Friis, Michael N Groves, Bjørk Hammer, Cory Hargus, *et al.*, "The atomic simulation environment — a Python library for working with atoms," Journal of Physics: Condensed Matter **29**, 273002 (2017).

[4] D Waasmaier and A Kirfel, "New analytical scattering-factor functions for free atoms and ions," Acta Crystallographica Section A: Foundations of Crystallography **51**, 416–431 (1995).
